# Supplementary material for: AndroCon: Conning Location Services in Android
Source: arXiv:2407.19392 source file (2024-07-28)
Supplement: Supplementary file 1 [file appendix.tex]

\section{appendix}
